# Supplementary material for: Time-Dependent Relativistic Two-Component Equation-of-Motion Coupled-Cluster for Open-Shell Systems: TD-EA/IP-EOMCC
Source: arXiv:2602.00985 ancillary file (2026-05-04)
Supplement: Supplementary file 1 [file td_ip_ea_eomcc_si.pdf]

# Supporting Information for: Time-Dependent Relativistic Two-Component Equation-of-Motion Coupled-Cluster for Open-Shell Systems: TD-EA/IP-EOMCC

P. D. Varuna S. Pathirage, Stephen H. Yuwono, and A. Eugene DePrince III[a)]

*Department of Chemistry and Biochemistry, Florida State University, Tallahassee, FL 32306-4390*

[a)]Electronic mail: adeprince@fsu.edu

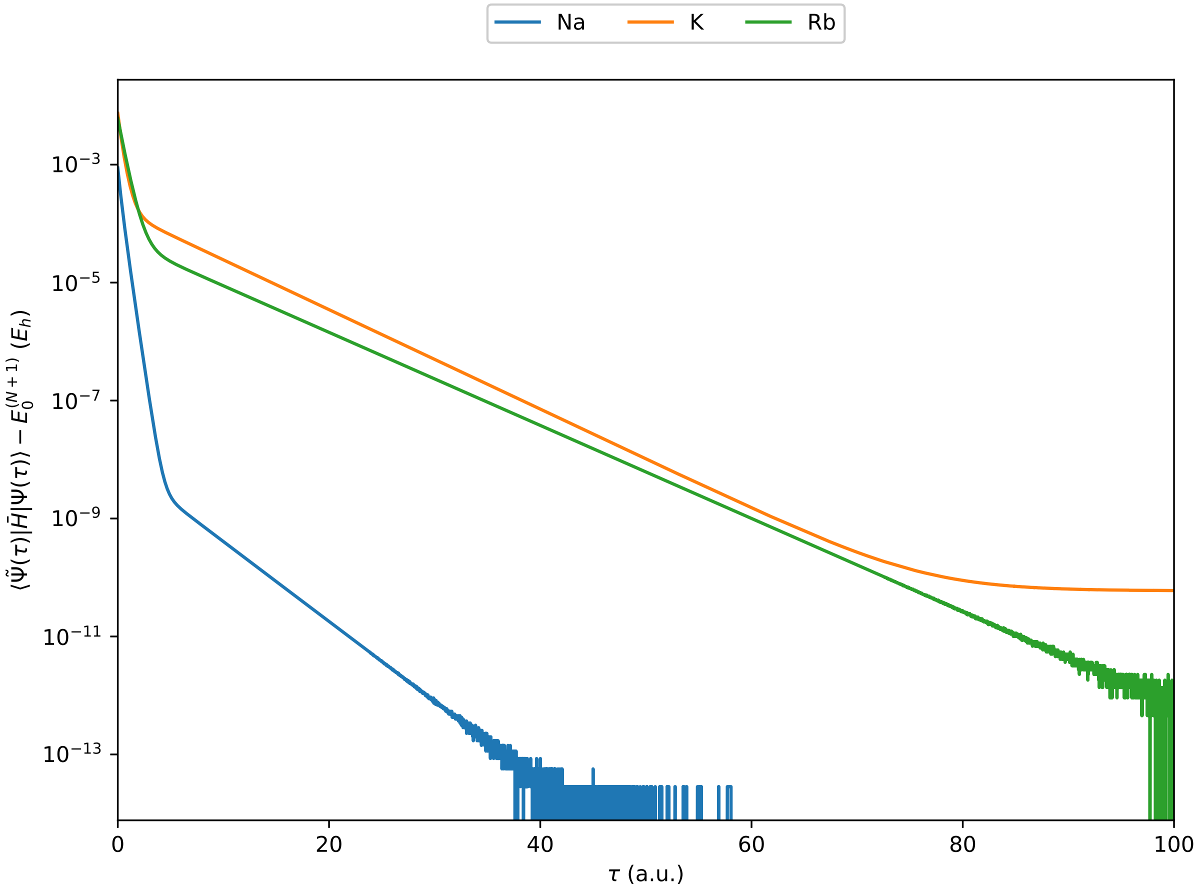


FIG. S1. Energy convergence for group I atoms with imaginary-time EA-EOMCCSD using a total propagation time of $\tau = 100.0$ a.u.

TABLE S1. Energy difference between the imaginary-time propagated state and the true open-shell ground state in $E_\mathrm{h}$. The frequency-domain EA/IP-EOMCCSD energy of the ground state of each atom is provided for reference.

| $\tau$ | $E(\tau)-E_0^{N+1}$ | | | $E(\tau)-E_0^{N-1}$ | | |
|---|---|---|---|---|---|---|
| | Na | K | Rb | F | Cl | Br |
| 0.0 | 0.000916 | 0.007643 | 0.006204 | 0.116961 | 0.055106 | 0.049263 |
| 2.5 | 0.000000 | 0.000122 | 0.000083 | 0.000002 | 0.000016 | 0.000065 |
| 5.0 | 0.000000 | 0.000064 | 0.000023 | 0.000000 | 0.000000 | 0.000000 |
| 7.5 | 0.000000 | 0.000039 | 0.000014 | 0.000000 | 0.000000 | 0.000000 |
| 10.0 | 0.000000 | 0.000024 | 0.000009 | 0.000000 | 0.000000 | 0.000000 |
| $E_0^{N\pm1}$ | −162.055590 | −601.465822 | −2979.028413 | −99.530985 | −460.907348 | −2604.389874 |

TABLE S2. Absolute values of the overlap between Koopman states and target EA/IP-EOMCCSD ground states (0) and between the Koopman states and the next lowest state with the same symmetry as the ground state ($K$) as a function of $\tau$. For each set of degenerate states, only the largest overlap is shown. See main text for the $0 \rightarrow K$ excitation energies.

| Atom | $\tau$ (a.u.) | $\lvert\langle\Phi^{(N\pm1)}\lvert\Psi_0^{(N\pm1)}\rangle\rvert$ | $\lvert\langle\tilde{\Psi}_0^{(N\pm1)}\lvert\Phi^{(N\pm1)}\rangle\rvert$ | $\lvert\langle\Phi^{(N\pm1)}\lvert\Psi_K^{(N\pm1)}\rangle\rvert$ | $\lvert\langle\tilde{\Psi}_K^{(N\pm1)}\lvert\Phi^{(N\pm1)}\rangle\rvert$ |
|---|---|---|---|---|---|
| Na | 0.0 | 0.999731 | 0.999770 | 0.000310 | 0.000155 |
| | 2.5 | 1.000000 | 1.000000 | 0.000210 | 0.000105 |
| | 5.0 | 1.000000 | 1.000000 | 0.000142 | 0.000071 |
| | 7.5 | 1.000000 | 1.000000 | 0.000096 | 0.000048 |
| | 10.0 | 1.000000 | 1.000000 | 0.000065 | 0.000033 |
| K | 0.0 | 0.996742 | 0.996484 | 0.041569 | 0.041667 |
| | 2.5 | 0.999455 | 0.999452 | 0.032658 | 0.032743 |
| | 5.0 | 0.999671 | 0.999669 | 0.025617 | 0.025684 |
| | 7.5 | 0.999797 | 0.999796 | 0.020092 | 0.020145 |
| | 10.0 | 0.999875 | 0.999875 | 0.015759 | 0.015800 |
| Rb | 0.0 | 0.996990 | 0.996402 | 0.011698 | 0.011600 |
| | 2.5 | 0.999778 | 0.999784 | 0.009339 | 0.009266 |
| | 5.0 | 0.999878 | 0.999880 | 0.007442 | 0.007384 |
| | 7.5 | 0.999923 | 0.999924 | 0.005931 | 0.005884 |
| | 10.0 | 0.999951 | 0.999952 | 0.004726 | 0.004689 |
| F | 0.0 | 0.665159 | 0.714051 | 0.000636 | 0.000593 |
| | 2.5 | 0.686414 | 0.724117 | 0.000018 | 0.000016 |
| | 5.0 | 0.686415 | 0.724117 | 0.000001 | 0.000000 |
| | 7.5 | 0.686415 | 0.724117 | 0.000000 | 0.000000 |
| | 10.0 | 0.686415 | 0.724117 | 0.000000 | 0.000000 |
| Cl | 0.0 | 0.686081 | 0.686156 | 0.000847 | 0.000785 |
| | 2.5 | 0.699121 | 0.694963 | 0.000059 | 0.000055 |
| | 5.0 | 0.699125 | 0.694967 | 0.000004 | 0.000004 |
| | 7.5 | 0.699125 | 0.694967 | 0.000000 | 0.000000 |
| | 10.0 | 0.699125 | 0.694967 | 0.000000 | 0.000000 |
| Br | 0.0 | 0.739439 | 0.712476 | 0.002724 | 0.002402 |
| | 2.5 | 0.732796 | 0.743009 | 0.000316 | 0.000294 |
| | 5.0 | 0.732816 | 0.743028 | 0.000037 | 0.000035 |
| | 7.5 | 0.732816 | 0.743028 | 0.000004 | 0.000004 |
| | 10.0 | 0.732816 | 0.743028 | 0.000001 | 0.000000 |

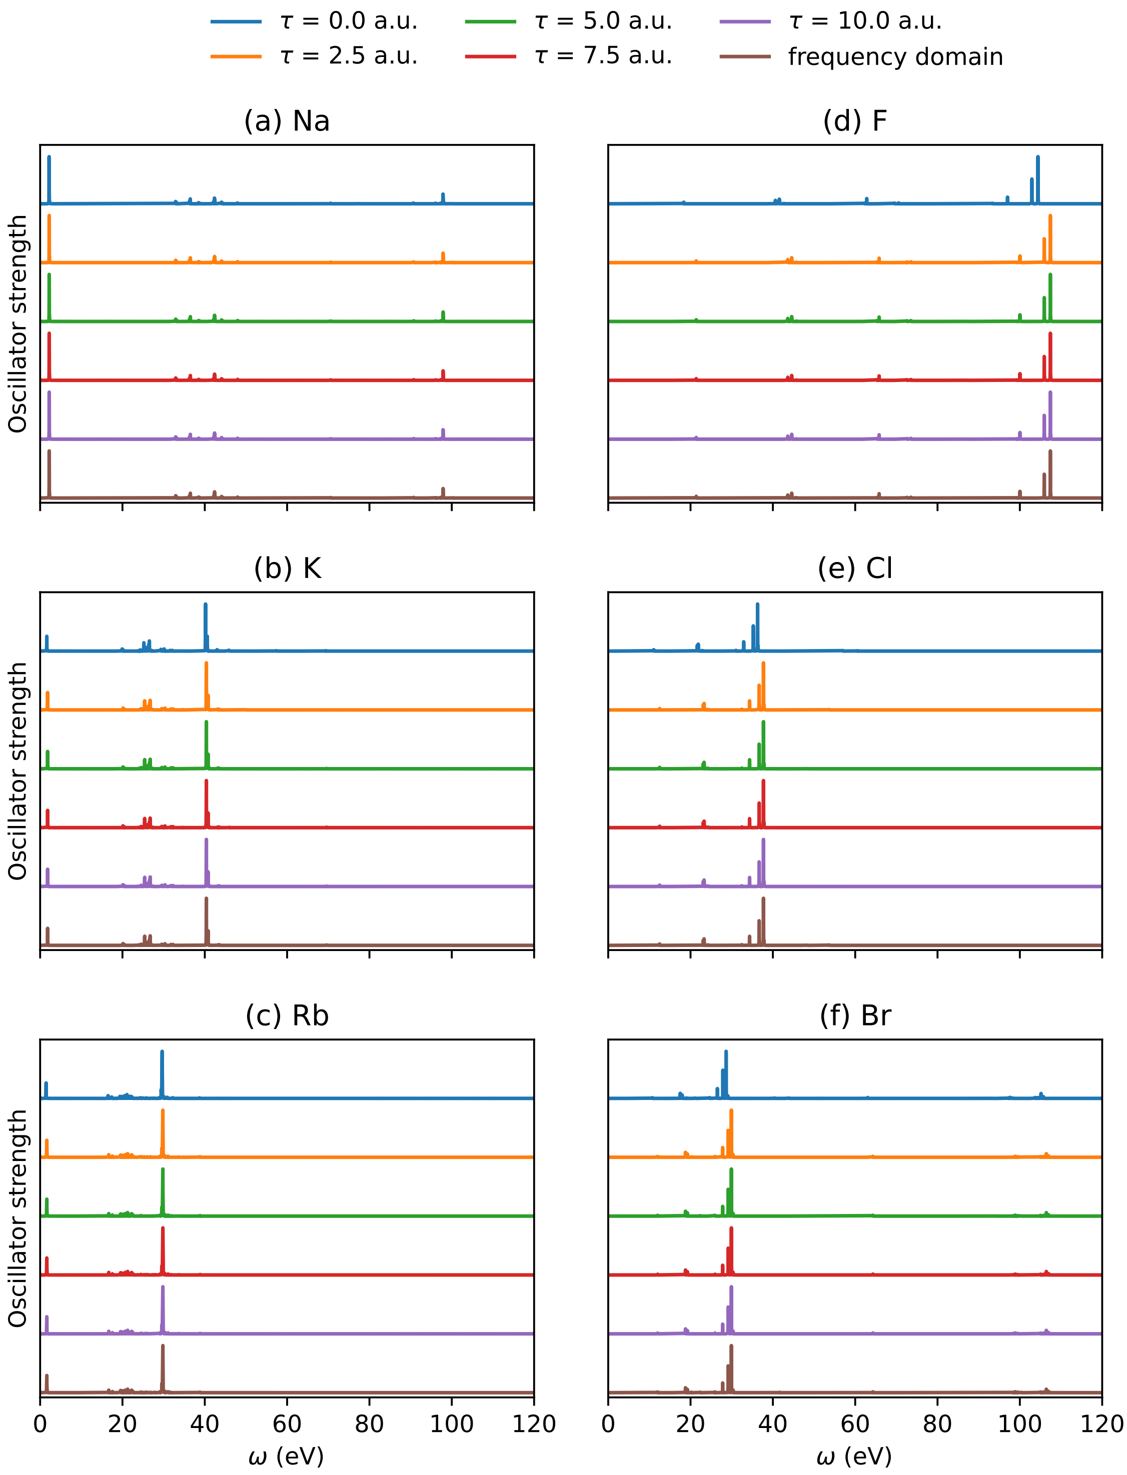


FIG. S2. Real-time spectrum obtained from Koopman state ($\tau = 0.0$, in blue), imaginary propagated states at $\tau = 2.5, 5.0, 7.5$ and 10.0 (in orange, green, red and purple respectively) and the frequency domain spectrum (in brown) for alkali metals and halogens. The peak heights are normalized to the highest intensity peak within the range 0 – 120 eV.
